# Supplementary material for: Forecasting Granular Audience Size for Online Advertising
Source: arXiv:1901.02412 source file (2019-01-08)
Supplement: Supplementary file 1 [file appendix.tex]

\appendix
\section*{Appendix}

\section{Attributes}\label{sec:appendix:attributes}
\subsection{Bid Requests dataset}
Here we describe briefly the categorical attributes that we used in the Bid Request dataset:
